# Supplementary material for: Antiferromagnetic Ground State of La$_{2}$CuO$_{4}$: A Parameter-free Ab Initio Description
Source: arXiv:1808.06283 ancillary file (2018-08-20)
Supplement: Supplementary file 1 [file Supplementary_Materials.pdf]

# Supplementary materials for: Antiferromagnetic Ground State of $La_2CuO_4$: A Parameter-free Ab Initio Description

Christopher Lane[1], James W. Furness[2], Ioana Gianina Buda[1], Yubo Zhang[2], Robert S. Markiewicz[1], Bernardo Barbiellini[3,1], Jianwei Sun[2], and Arun Bansil[1]
[1]*Physics Department, Northeastern University, Boston MA 02115, USA*
[2]*Department of Physics and Engineering Physics, Tulane University, New Orleans, LA 70118, USA*
[3]*Department of Physics, School of Engineering Science, Lappeenranta University of Technology, FI-53851 Lappeenranta, Finland*

(Dated: version of August 19, 2018)

## I. DFT AS A MANY-ELECTRON THEORY AND INTRINSIC LIMITATIONS OF THE BAND THEORY PARADIGM

In the early 1900's the Schrodinger equation for quantum wavefunctions had already proven highly accurate for simple systems like He and $H_2$, prompting Dirac to declare "chemistry had come to an end–its content was entirely contained in that powerful equation"[1]. However, in almost all practical cases the many-body Schrodinger equation is far too complex to solve. The transformational insight of Kohn[2,3] was to take a different approach by considering the *density* rather than the wavefunction as the fundamental object for addressing the many-body problem. thus, the density functional theory (DFT) is not designed for obtainging wavefunctions in its basic construction. DFT is a formally rigorous approach to treat *any* interacting system by mapping it onto a non-interacting system for its ground state properties[4], and it is thus obviously not a one-electron theory.

The misunderstanding about the DFT being a one-particle theory has been driven in part by the inability of the existing density functionals to describe correctly the ground state of some strongly-correlated materials. But, the DFT can, in principle, provide an exact description of the ground state and related physical properties of any material, regardless of the strength of the correlations. The many-body effects are incorporated in the DFT through the treatment of the exchange-correlation energy ($E_{xc}$), which in practice must be approximated. We emphasize that even though single-determinant wavefunctions are invoked prominently in the DFT and give the theory an appearance of being a one-particle theory, these single-determinant wavefunctions only serve as auxiliary quantities, which provide a natural starting point for incorporating many-body effects in the theory.

The key is to recognize that the DFT maps the interacting many-electron Hamiltonian in a solid onto an effective non-interacting one-electron Hamiltonian, which is rigorously justified insofar as the ground state energy is concerned. However, the associated one-electron Kohn-Sham energies/orbitals, which are the basis of the common band structures that have come to symbolize band theory so vividly, do not represent the physically relevant quasiparticles of the many-electron system. Even the exact exchange-correlation functional for this reason should not be expected to provide the quasiparticle spectrum of the electron gas. [Notably, time-dependent generalization of the DFT (TDDFT) can, in principle, provide an exact treatment of the excited states.]

Despite lack of a link with quasiparticles, Kohn-Sham one-particle Bloch states have assumed a commanding air of 'reality' over the years and provided an effective basis for coding the essence of the 'genome' of a material. The reason is that many experiments, including direct mapping of bands several volts deep in the Fermi sea via angle-resolved photoemission experiments, show clearly that the Bloch states and the related energies and Fermi surfaces predicted by the DFT are in remarkable accord with experiments in wide classes of materials. Such band structures are being used extensively for designing myriad devices for technological applications, and have resulted in the successful prediction of most known topological materials, from insulators to Weyl semi-metal phases, before these topological materials were actually realized experimentally[5].

All materials are correlated because electrons confined to lattice dimensions will generally experience quite strong Coulomb forces. The success of the band theory in many materials where the DFT captures measured properties of quasiparticles with remarkable accuracy then suggests that Bloch states in these cases reasonably approximate quasiparticles. It is not unreasonable then to expect that as the description of the ground state energy improves with the use of improved density functionals, we will also see that the Bloch states better mimic the quasiparticles.

The preceding discussion clearly suggests that the Bloch states produced by SCAN are a better representation of quasiparticles in the cuprates compared to those generated by any other existing density functional. On the other hand, the band theory paradigm as it is practiced currently will never be able to model certain properties of the quasiparticles. For example, the spectral function for Bloch electrons consists of $\delta$-functions with uniform spectral

weights, but that is not the case in the cuprates where the quasiparticles exhibit finite lifetimes and non-linear evolutions in spectral weights with doping, and spectral functions that contain coherent and incoherent parts in general.[6]

Despite the limitations inherent to the band theory framework itself, the ability of the SCAN functional to capture the ground state of LCO and its many key properties opens the door for the first time for parameter-free first-principles modeling of electronic structures of cuprates and other materials that have been considered to be so strongly correlated as to lie outside the scope of the DFT.

## II. TECHNICAL ASPECTS OF THE IMPLEMENTATION OF META-GGA EXCHANGE-CORRELATION FUNCTIONALS

The SCAN functional avoids dependence on the density Laplacian in favor of the orbital kinetic energy density in its construction. Moreover, SCAN involves only the orbital kinetic energy density as information beyond the GGA. Although functionals invoking the density Laplacian have generally been taken to belong to the 'meta-GGA' classification, the orbital kinetic energy density is the more commonly accepted ingredient in meta-GGA functionals. We employ the method of Handy's group[7] in which the total energy is minimized with respect to the occupied orbitals and yields an effective orbital-dependent potential. The technique of partial integration is further employed in VASP to avoid requiring higher derivatives of the basis set. These techniques are also summarized in Ref. 8.

Numerically, the SCAN functional is sensitive to real-space grid density[9]. We have thoroughly checked the convergence of all our results with respect to grid densities. Notably, the sensitivity of the SCAN functional to the grid density reflects the presence of fine structure in the potential, and not the use of high-order derivatives. As we sample diverse chemical environments in a crystal, the SCAN potential undergoes dramatic changes as it attempts to accommodate rapid variations in the types of bondings involved, especially in the inter-shell regions. This in turn drives fine structures in the SCAN potential.

## III. COMPARISON BETWEEN LSDA/GGA AND SCAN BASED BAND GAPS AND ELECTRONIC STRUCTURES

The physical interpretation of the band gap obtained in the ground state DFT calculations has been the subject of much debate in the literature over the years. In comparing the band structures based on different functionals one must distinguish between the nature of the effective exchange-correlation potential obtained in the Kohn-Sham (KS) and generalized Kohn-Sham (gKS) formalisms underlying the construction of various functionals. KS potentials are 'multiplicative' by design in that they are orbital-independent. In sharp contrast, gKS potentials are formally constructed with the freedom to be orbital-dependent and can thus be 'non-multiplicative'.

In particular, LSDA/GGA band structures involve multiplicative effective potentials, while the current and common SCAN implementations involve non-multiplicative potentials due to the inclusion of the kinetic energy density as an ingredient, and thus differ in their basic underlying designs.

In this connection, Perdew et. al.[10] have shown recently that for a given density functional, the gKS band gap is equal to the fundamental band gap in the solid, which is defined as the ground state energy difference between systems with different number of electrons. There is thus a firm basis for comparing computed band gaps within the gKS-based SCAN formalism with the experimentally observed band gaps (excluding excitonic effects). The preceding considerations indicate that as a meta-GGA functional improves the description of the ground state, it will necessarily also lead to improvement in the band gap.

Table S1 compares the magnetic moments and band gaps of LCO for various meta-GGA DFT functionals. Here we tested popular meta-GGA functionals available in VASP including M06L[11], TPSS[12] and revTPSS[13]. M06L is widely used in chemistry and is heavily parameterized, which leads to well known numerical stability problems (a consequence of overfitting)[14]. Our calculations confirm this point. TPSS and revTPSS are earlier versions of the non-empirical meta-GGAs, which are seen to underestimate the magnetic moment, and give only slight improvement over PBE. Overall, the best results are found with SCAN.

TABLE S1. Comparison of theoretically predicted magnetic movements and bands gaps of low-temperature orthorhombic (LTO) phase of $La_2CuO_4$ using various meta-GGA functionals.

| Functional | Cu Magnetic Moment ($\mu_B$) | Band Gap (eV) |
|---|---|---|
| M06L | Unable to converge due to numerical instabilities | |
| revTPSS | 0.320 | 0.21 |
| TPSS | 0.313 | 0.18 |
| SCAN | 0.490 | 1.0 |

## IV. OPTICAL SPECTRA

In estimating the band gap from the optical spectra for the half-filled system given in Fig. 4 of Ref. 15, we should be careful to look for the leading edge gap in the spectrum, which yields the value of 0.91 eV that is in good accord with our predicted value of 1.0 eV in LCO, excitonic effects notwithstanding. In particular, the first peak in the optical spectrum above the Fermi energy is not a good marker for estimating the band gap. Note also that the weak mid-infrared features in the optical spectra of cuprates, reported in some nominally undoped samples, have been interpreted mainly in terms of residual impurities. Although scanning-tunneling spectroscopy (STS) has not been successful on LCO, a large charge gap in good agreement with our results has been observed in STS studies in a closely-related cuprate; in-gap features were observed, but only in the vicinity of impurities[16]. Transport studies find similar gap values, suggesting an absence of mobile mid-infrared carriers[17]. We have carried out modeling of the optical spectra of the cuprates, and shown that the computed spectrum reasonably reproduces the measured spectrum in the half-filled cuprates with a leading edge gap of about 1 eV, see Ref. 18 for details.

## V. EXPERIMENTAL COPPER MAGNETIC MOMENTS

Table S2 compares copper magnetic moment values from various experiments, including the value given in the recent review of Tranquada[19]. The considerable variability in the values stems from variations in sample quality and the approximate nature of the form factors used in calculating the copper magnetic moment. We hope that our first-principles form factor present in this study will aid in obtaining improved experimental magnetic moment values.

TABLE S2. Experimental copper magnetic moments of AFM $La_2CuO_4$ obtained via neutron scattering measurements. The magnetic form factor used in calculating the magnetic moment is indicated in those cases where it is available.

| Experimental Technique | Cu Magnetic Moment ($\mu_B$) | Reference | Form Factor |
|---|---|---|---|
| Neutron Diffraction (Powder) | 0.48±0.15 | 20 | f(Q)=0.75 ($K_2CuF_4$)[21] |
| Neutron Diffraction (Powder) | 0.4 | 20 | $Cu^{++}$ |
| Neutron Diffraction (Powder) | 0.43±0.13 | 22 | f(Q)=0.75 ($K_2CuF_4$)[21] |
| Neutron Diffraction (Single Crystal) | 0.35±0.05 | 23 | N/A |
| Neutron Diffraction (Single Crystal) | 0.60±0.05 | 24 | f(100)=0.835 ($K_2CuF_4$)[25] |
| Neutron Diffraction (Single Crystal) | 0.30 | 26 | f(100)=0.835 ($K_2CuF_4$)[25] |
| Neutron Diffraction (Single Crystal) | 0.40 | 27 | N/A |

## VI. DETAILS OF CRYSTAL STRUCTURE

TABLE S3. Theoretical and experimental lattice parameters, volume and Wyckoff positions for atomic sites in the low temperature orthorhombic (LTO) phase of $La_2CuO_4$. The calculated structural data are in agreement with the *Bmab* symmetry found experimentally.

| | | Experiment[a] | Present Theory |
|---|---|---|---|
| $a$ (Å) | | 5.3350 | 5.324 |
| $b$ (Å) | | 5.4209 | 5.458 |
| $c$ (Å) | | 13.1068 | 13.087 |
| $V$ (Å$^2$) | | 379.0552 | 380.313 |
| La | $x$ | 0 | 0 |
| | $y$ | 0.0092 | 0.0117 |
| | $z$ | 0.3618 | 0.3608 |
| Cu | $x = y = z$ | 0 | 0 |
| O(1) | $x = y$ | 0.25 | 0.25 |
| | $z$ | 0.0085 | 0.0113 |
| O(2) | $x$ | 0 | 0 |
| | $y$ | -0.0426 | -0.0562 |
| | $z$ | 0.1839 | 0.1858 |
| Octahedral tilt (°)[b] | O(1) | 3.3532 | 4.4538 |
| | O(2) | 5.4727 | 7.1971 |

[a] Experimental structural data are taken from Ref. 28 as stated in Ref. 29.
[b] The tilt angle is measured off of the ab-plane and the c-axis for O(1) and O(2) , respectively. The calculated tilt angles are consistent with the results of Refs. 30 and 27.

## VII. MOLECULAR-BONDING PICTURE OF OCTAHEDRALLY COORDINATED Cu IN $La_2CuO_4$

Fig. S1 shows a schematic of the molecular-bonding picture of octahedrally coordinated Cu in $La_2CuO_4$, which is adapted from that presented in Refs.31 and 32. A sketch of the atomic positions is given in the top portion of the figure, where Cu and O atoms are shown in red and teal colors, respectively. The atomic Cu 3d levels in an octahedral crystal field split into $e_g$ and $t_{2g}$ manifolds. A tetragonal Jahn-Teller distortion splits the $e_g$ and $t_{2g}$ states along with the O 2p states, as shown. In the central portion of the figure, we show the resulting hybridized complex of states, along with the separation of the bonding ($\sigma$) and antibonding ($\sigma^*$) states for $d_{x^2-y^2}$ and $d_{z^2}$ orbitals. The $d_{z^2}$ bonding and antibonding states have been included due to their sizable contribution to the valence states in the AFM phase as discussed in the main text.

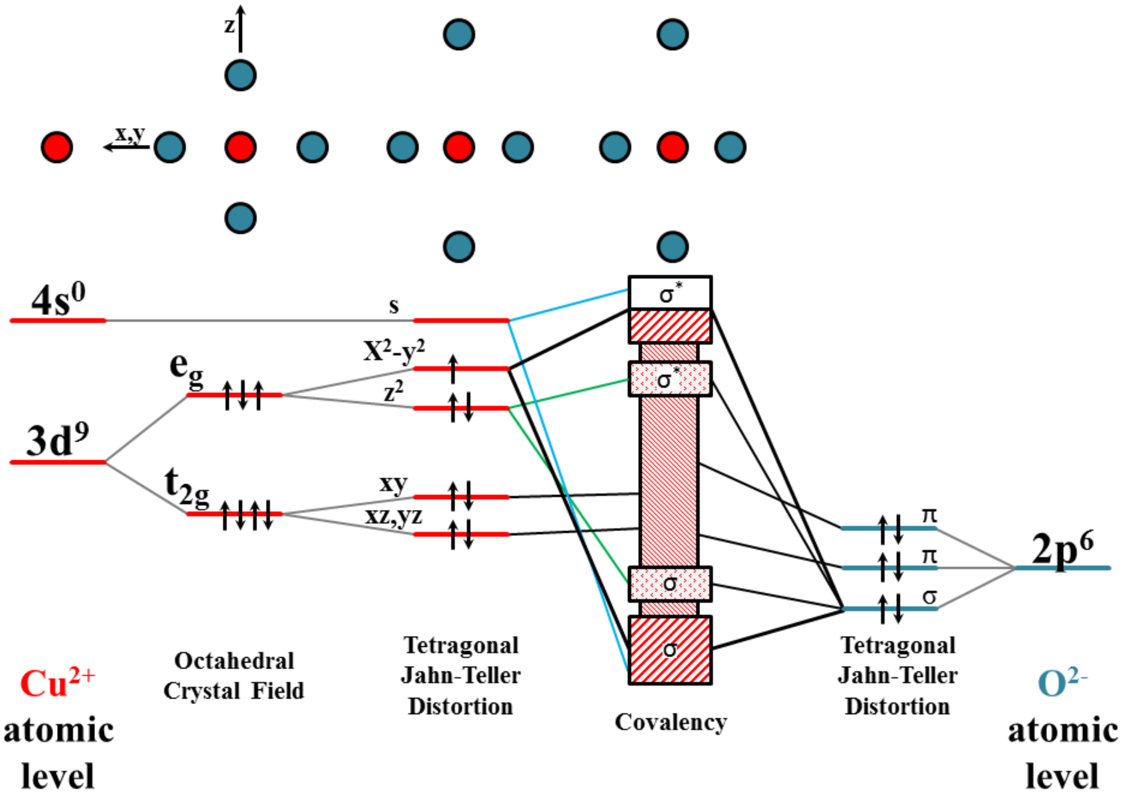


FIG. S1. The schematic molecular-bonding picture of octahedrally coordinated Cu discussed in the text.

## VIII. HUND'S SPLITTING IN $La_2CuO_4$ AND ESTIMATES OF $U$ AND $J_H$ INTERACTIONS

Since our first-principles computations correctly capture the AFM ground state without invoking any empirical parameters, we can estimate the effective values of the multi-orbital interactions from our ground state electronic structure. Let us first consider an orbital $\mu$ in a ligand field. The energy of this orbital will be split into a pair of bonding and anti-bonding states with energies:

$$E^{\mu\sigma}_{\pm} = a^{\pm}_{\mu\sigma} \pm h_{\mu} \tag{1}$$

where $\pm$ indexes the bonding $(-)$ and anti-bonding $(+)$ states, $h$ is the hybridization strength, and $a^{\pm}_{\mu\sigma}$ is the bare orbital energy. The bare orbital energy can be broken down into two terms, an on-site atomic term, and an interaction term:

$$a^{\pm}_{\mu\sigma} = E^{\mu}_{Atomic} + H^{\mu\sigma\pm}_{int} \tag{2}$$

For the form of $H^{\mu\sigma\pm}_{int}$ we will follow Oles[33], whereby we only consider electron correlations in the $3d$ orbitals, and the electron-electron interactions are restricted to be intra-site, in agreement with Hubbard. In order to make the model tractable, we work in the mean-field where an electronic state is influenced by the presence of other electrons via the effective field $H_{\mu\sigma}$

$$H_{\mu\sigma} = U\langle n_{\mu\bar{\sigma}}\rangle + \sum_{\nu\neq\mu} U'\langle n_{\nu\bar{\sigma}}\rangle + \sum_{\nu\neq\mu}(U' - J_H)\langle n_{\nu\sigma}\rangle, \tag{3}$$

with orbital $(\mu, \nu)$ and spin $(\sigma, \bar{\sigma} = -\sigma)$ indices, and $\langle n_{\mu\sigma}\rangle$ is the average electron occupation for a given state. Therefore, we can insert $H_{\mu\sigma}$ from Eq.3 into Eq.,

$$a^{\pm}_{\mu\sigma} = E^{\mu}_{Atomic} + U\langle n^{\pm}_{\mu\bar{\sigma}}\rangle + U'\sum_{\nu\neq\mu}\langle n^{\pm}_{\nu\bar{\sigma}}\rangle + (U' - J_H)\sum_{\nu\neq\mu}\langle n^{\pm}_{\nu\sigma}\rangle \tag{4}$$

Since our main interest is to extract the interaction parameters, i.e. $U$ and $J_H$, we take the difference between spin configurations and sum over bonding and anti-bonding states to eliminate the hybridization and atomic contributions, which are assumed to be spin-independent, yielding:

$$E^{\mu\uparrow} - E^{\mu\downarrow} = \sum_{\pm} E^{\mu\uparrow}_{\pm} - E^{\mu\downarrow}_{\pm} = \sum_{\pm}(a^{\pm}_{\mu\uparrow} - a^{\pm}_{\mu\downarrow}) \tag{5}$$

$$= \sum_{\pm}[(U\langle n^{\pm}_{\mu\downarrow}\rangle + U'\sum_{\nu\neq\mu}\langle n^{\pm}_{\nu\downarrow}\rangle + (U' - J_H)\sum_{\nu\neq\mu}\langle n^{\pm}_{\nu\uparrow}\rangle)$$

$$- (U\langle n^{\pm}_{\mu\uparrow}\rangle + U'\sum_{\nu\neq\mu}\langle n^{\pm}_{\nu\uparrow}\rangle + (U' - J_H)\sum_{\nu\neq\mu}\langle n^{\pm}_{\nu\downarrow}\rangle)] \tag{6}$$

$$= U(N_{\mu\downarrow} - N_{\mu\uparrow}) + U'\sum_{\nu\neq\mu}(N_{\nu\downarrow} - N_{\nu\uparrow}) + (U' - J_H)\sum_{\nu\neq\mu}(N_{\nu\uparrow} - N_{\nu\downarrow}) \tag{7}$$

Here, $N_{\mu\sigma} = \sum_{\pm}\langle n^{\pm}_{\mu\sigma}\rangle$ is the total number of electrons in orbital $\mu$ of spin $\sigma$.

After hybridization, energy levels $E^{\mu\sigma}$ need not be localized in energy and may be smeared. With this in mind, we interpret $E^{\mu\sigma}$ as the average level energy, and write $E^{\mu\sigma}$ with respect to the density-of-states as

$$E^{\mu\sigma} = \int_W g_{\mu\sigma}(e)e\, de \tag{8}$$

where $W$ is the band width. Moreover, $E^{\mu\uparrow} - E^{\mu\downarrow}$ can be written as

$$E^{\mu\uparrow} - E^{\mu\downarrow} = \int_W g_{\mu\uparrow}(e)e - g_{\mu\downarrow}(e)e\, de. \tag{9}$$

Thus, we arrive at a linear set of equations indexed by $\mu$ relating the average orbital spin-splitting and the mean-field multi-orbital interactions,

$$\int_W g_{\mu\uparrow}(e)e - g_{\mu\downarrow}(e)e\, de = U(N_{\downarrow} - N_{\uparrow}) + U'\sum_{\nu\neq\mu}(N_{\nu\downarrow} - N_{\nu\uparrow}) + (U' - J)\sum_{\nu\neq\mu}(N_{\nu\uparrow} - N_{\nu\downarrow}). \tag{10}$$

Specifically, using the copper-atom-projected partial-density-of-states in the AFM phase of LTO $La_2CuO_4$ in Fig.S2(a), we find $N_{d_{x^2-y^2}\downarrow} - N_{d_{x^2-y^2}\uparrow} = 1/2$, and 0 for all other orbitals (using $\int de \sum_\sigma g_{\mu\sigma}(e)$ normalized to 1.0). This significantly simplifies Eq.10 to

$$\int_W g_{d_{x^2-y^2}\uparrow}(e)e - g_{d_{x^2-y^2}\downarrow}(e)e\, de = U(1/2) \tag{11}$$

$$\int_W g_{d_{z^2}\uparrow}(e)e - g_{d_{z^2}\downarrow}(e)e\, de = U'(1/2) + (U' - J)(-1/2) = J \tag{12}$$

$$\int_W g_{d_{xy}\uparrow}(e)e - g_{d_{xy}\downarrow}(e)e\, de = U'(1/2) + (U' - J)(-1/2) = J \tag{13}$$

$$\int_W g_{d_{xz}\uparrow}(e)e - g_{d_{xz}\downarrow}(e)e\, de = U'(1/2) + (U' - J)(-1/2) = J \tag{14}$$

$$\int_W g_{d_{zy}\uparrow}(e)e - g_{d_{zy}\downarrow}(e)e\, de = U'(1/2) + (U' - J)(-1/2) = J \tag{15}$$

Furthermore, we compute $\int_W g_{\mu\uparrow}(e)e - g_{\mu\downarrow}(e)e\, de$ for each orbital (cumulative sum seen in Fig.S2(b)). The average splitting calculated for $d_{x^2-y^2}$, $d_{z^2}$, $d_{yz}$, $d_{xz}$, and $d_{xy}$ is 2.423 eV, 0.624 eV, 0.424 eV, 0.424 eV, and 0.0195 eV, respectively.[34] Interestingly, we find a strong orbital dependence of the spin-splitting. Using our first-principles splittings, we estimate $U$ as $2.423/0.5 = 4.846$ eV. In estimating $J_H$ we take the largest splitting as an upper-bound on $J_H$, and obtain $J_H$ as $0.624/0.5 = 1.248$ eV.

In summary, we find strong orbital-dependent average spin splittings allowing us to estimate the multi-orbital interaction strengths to be $U = 4.846$ eV and $J_H = 1.248$ eV. We find considerable Hund's splitting, which is important for building accurate low-energy models of the electronic structure.

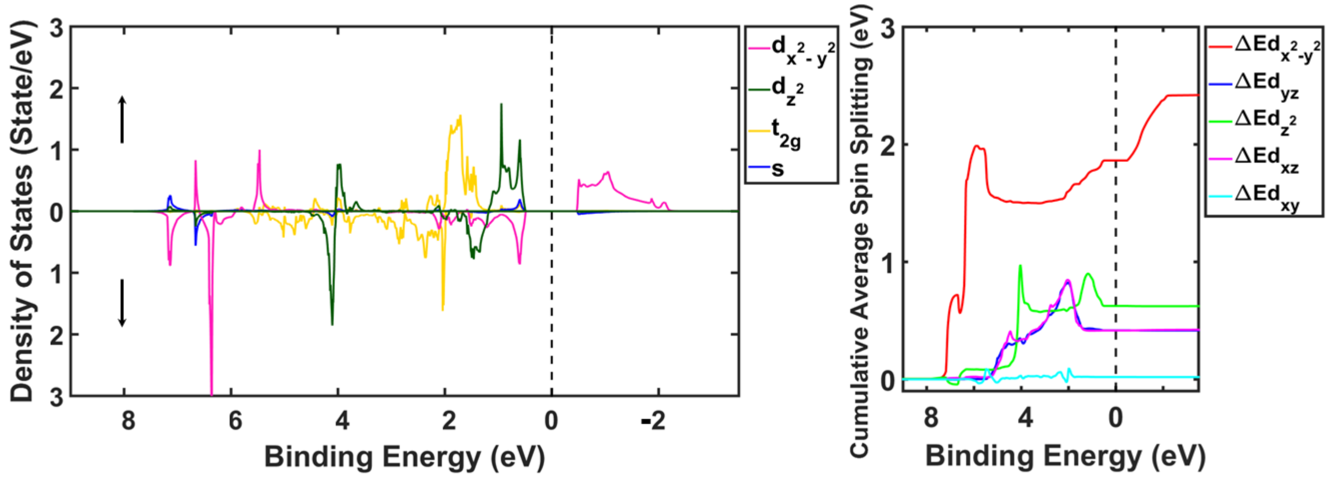


FIG. S2. (color online) (a) Single Copper site-resolved partial densities of states in the antiferromagnetic (AFM) phase of LTO $La_2CuO_4$. Copper d-orbital characters are plotted in various colors (see legend). (b) Cumulative average spin-splitting energies calculated for various d-orbitals for a single copper site.

## IX. DETAILS OF THE GAP AT 1.0 eV BINDING ENERGY

Fig. S3 presents the band structure (blue lines) of $La_2CuO_4$ in the LTO structure in the nonmagnetic (NM) and antiferromagnetic (AFM) states, overlaid with site-resolved atomic projections (red dots) for Cu $d_{x^2-y^2}$ and Cu $d_{z^2}$. Sizes of red dots are proportional to the fractional weights of indicated orbitals. The corresponding projected DOS's for the NM and AFM state are given at the periphery of the figure on the left and right hand sides, respectively. Comparing $d_{x^2-y^2}$ and $d_{z^2}$ weights, an avoided crossing is seen at 1.5 eV binding energy in the NM state which continues in the AFM state. The 0.16 eV gap at 1 eV binding energy can be seen in the AFM state, breaking the band degeneracy of the $d_{z^2}$ states in the NM phase.

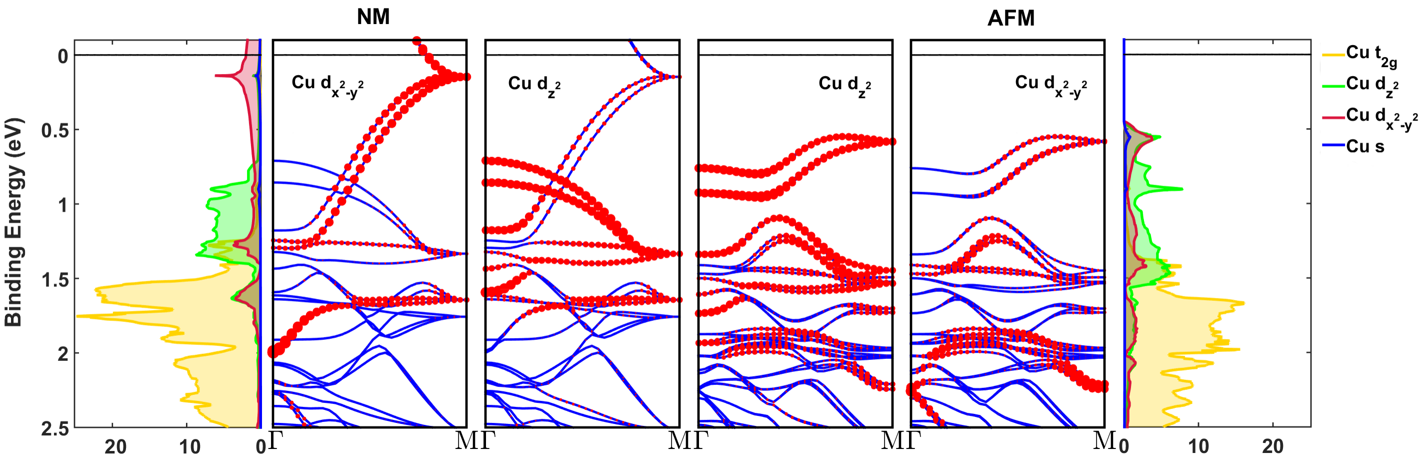


FIG. S3. Band structures for the NM and AFM phases of $La_2CuO_4$ and related orbital contributions for understanding details of the gap at 1 eV binding energy discussed in the text.

## X. NM AND AFM BAND STRUCTURES AND THEIR ORBITAL PROJECTIONS

Figs. S4-S11 give band structures (blue lines) of $La_2CuO_4$ in the LTO crystal structure for the nonmagnetic (NM) and antiferromagnetic (AFM) states overlaid with various site-resolved atomic projections (red dots).

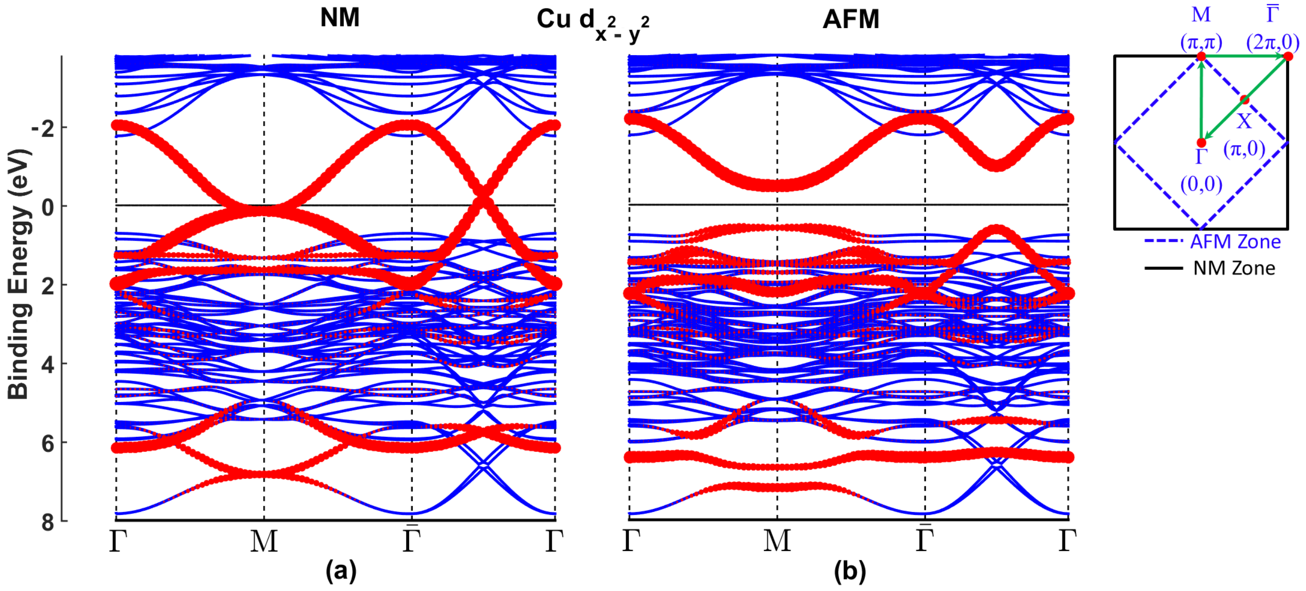


FIG. S4. Band structures (blue lines) along high-symmetry lines in the Brillouin zone in the NM and AFM phases of $La_2CuO_4$ in the LTO crystal structure. Contribution of Cu $d_{x^2-y^2}$ orbitals is highlighted with red dots. Sizes of red dots are proportional to the fractional weights of the Cu $d_{x^2-y^2}$ orbital in the corresponding crystal wavefunctions. A schematic diagram of the NM and AFM Brillouin zones with the path followed in presenting the band structures is shown on the right.

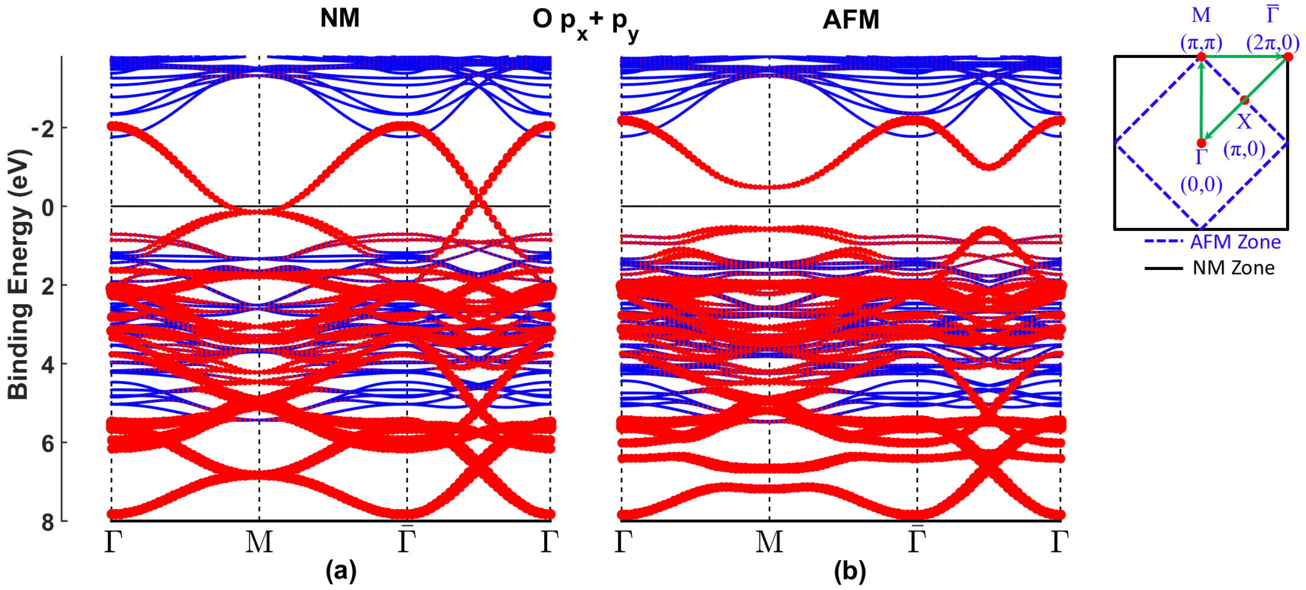


FIG. S5. Same as the caption to Fig. S4, except that this figure refers to O $p_x$+$p_y$ orbital contributions to the band structures.

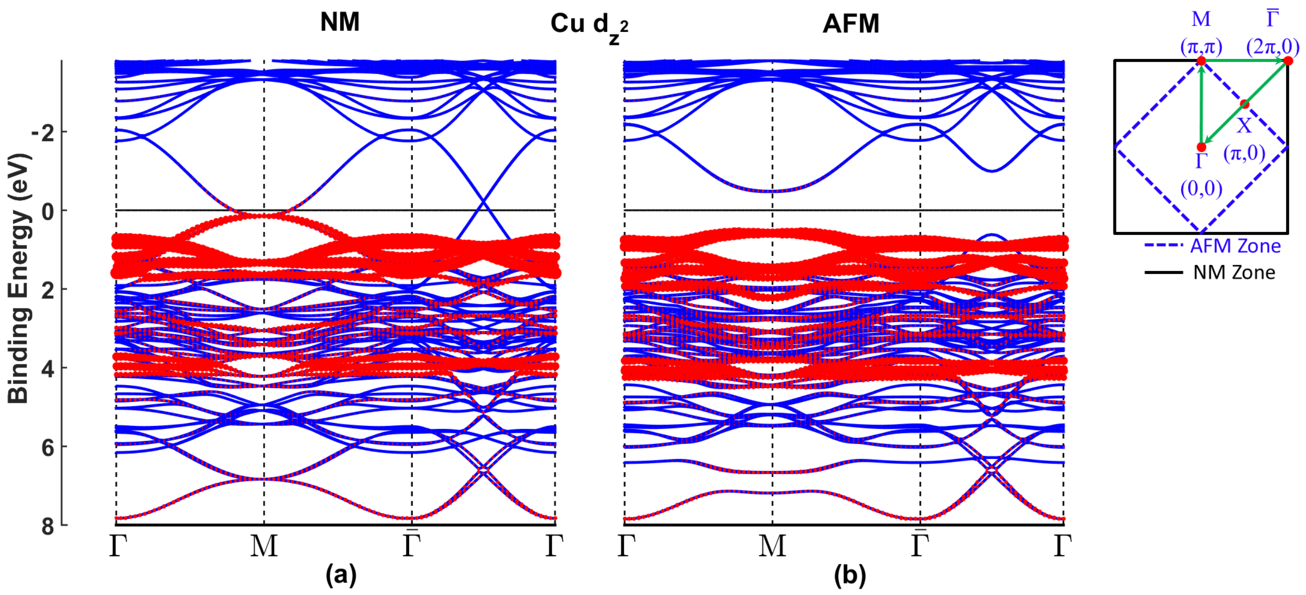


FIG. S6. Same as the caption to Fig. S4, except that this figure refers to Cu $d_{z^2}$ orbital contributions to the band structures.

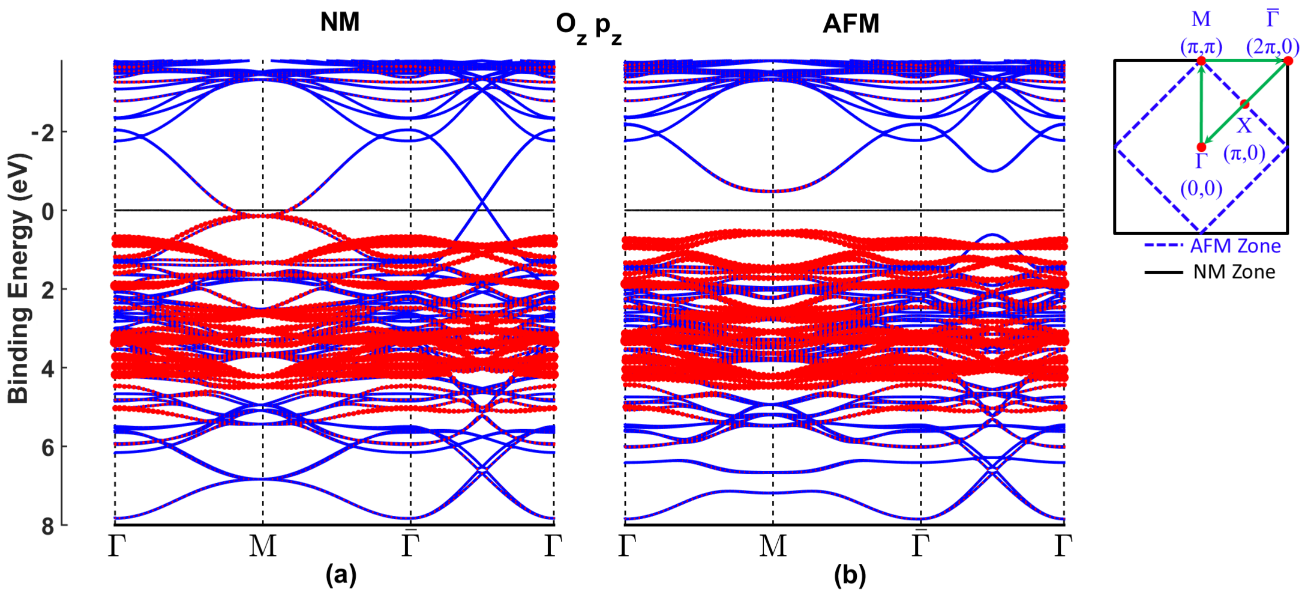


FIG. S7. Same as the caption to Fig. S4, except that this figure refers to $O_z$ $p_z$ orbital contributions to the band structures.

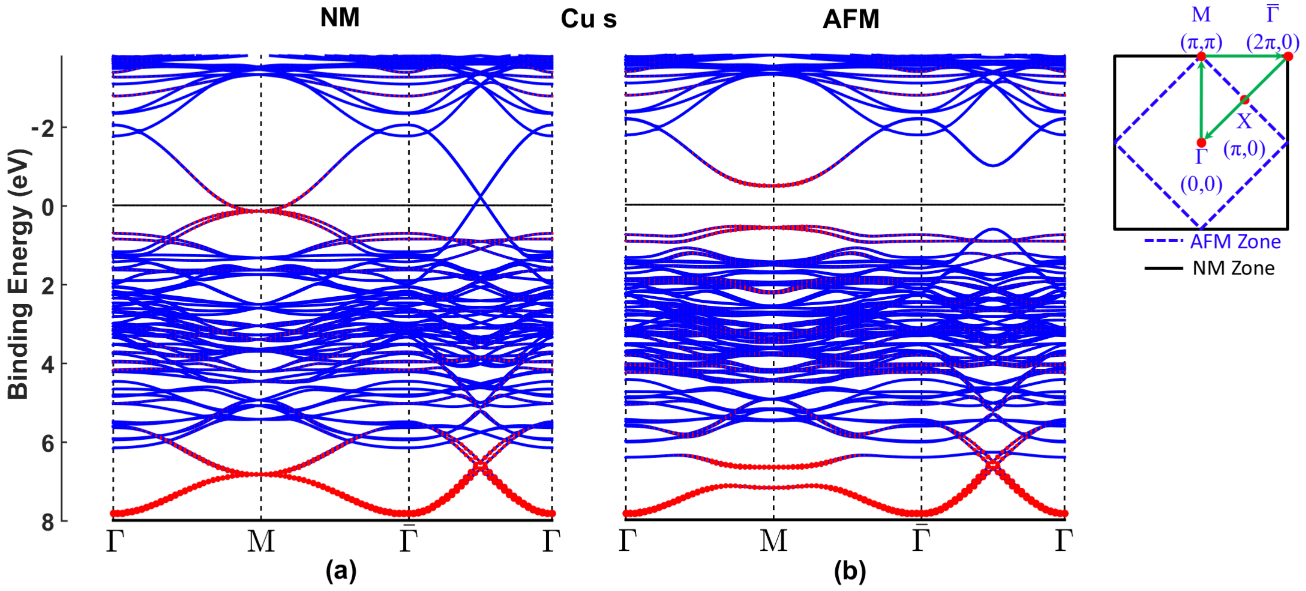


FIG. S8. Same as the caption to Fig. S4, except that this figure refers to Cu $s$ orbital contributions to the band structures.

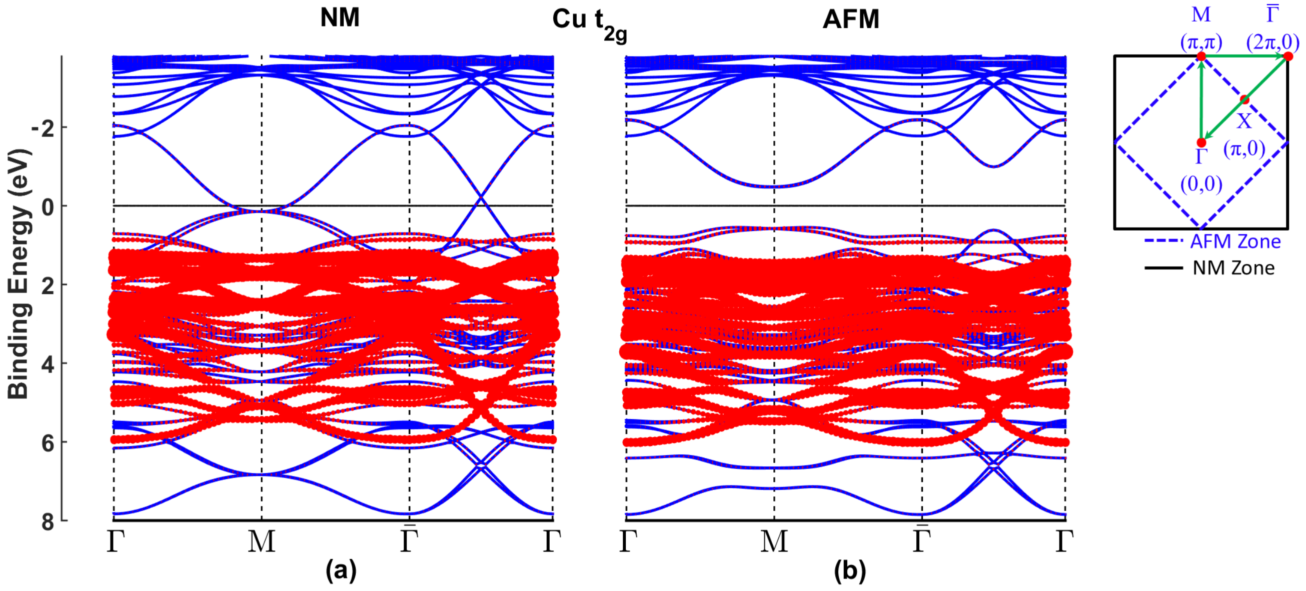


FIG. S9. Same as the caption to Fig. S4, except that this figure refers to Cu $t_{2g}$ orbital contributions to the band structures.

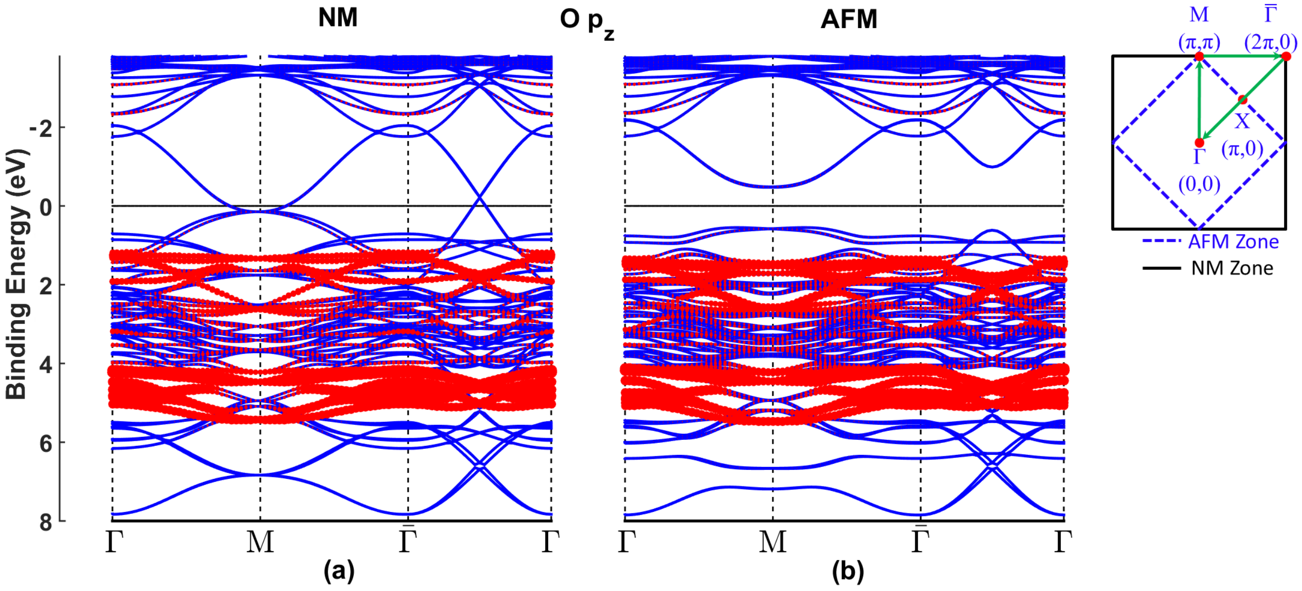


FIG. S10. Same as the caption to Fig. S4, except that this figure refers to O $p_z$ orbital contributions to the band structures.

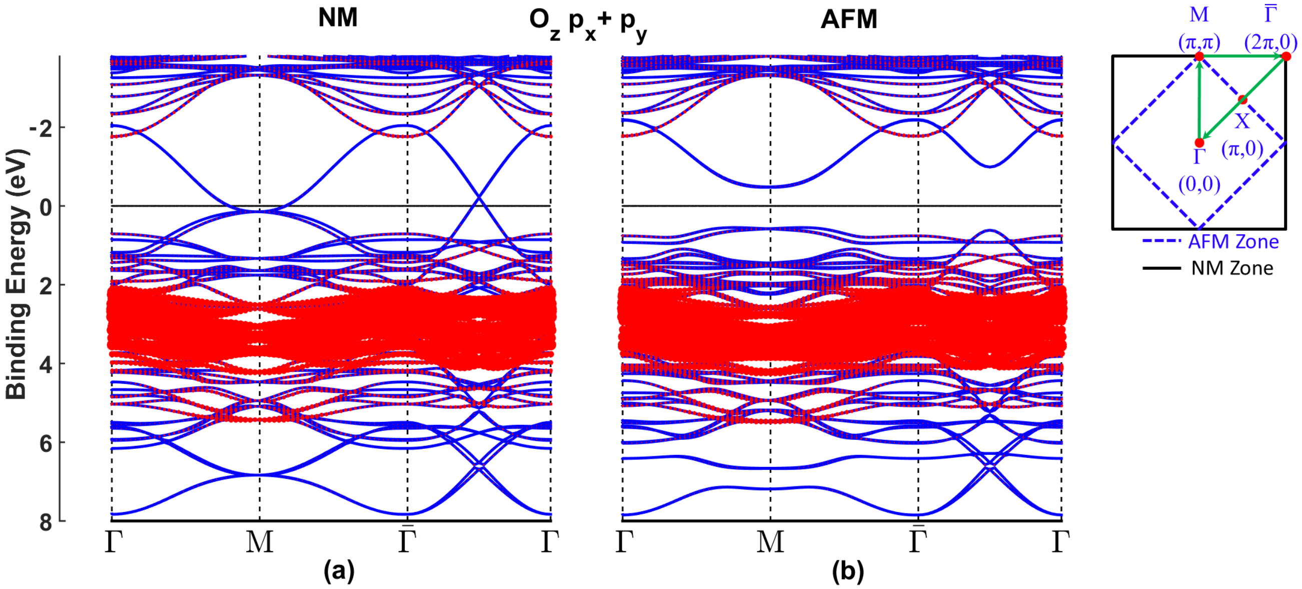


FIG. S11. Same as the caption to Fig. S4, except that this figure refers to $O_z$ $p_x$+$p_y$ orbital contributions to the band structures.

[1] W. Kohn, Reviews of Modern Physics **71**, 1253 (1999).
[2] P. Hohenberg and W. Kohn, Physical Review **136**, B864 (1964).
[3] W. Kohn and L. J. Sham, Physical Review **140**, A1133 (1965).
[4] K. Burke *et al.*, Department of Chemistry, University of California , 40 (2007).
[5] A. Bansil, H. Lin, and T. Das, Reviews of Modern Physics **88**, 021004 (2016).
[6] T. Das, R. S. Markiewicz, and A. Bansil, Advances in Physics **63**, 151 (2014).
[7] R. Neumann, R. H. Nobes, and N. C. Handy, Molecular Physics **87**, 1 (1996).
[8] J. Sun, M. Marsman, G. I. Csonka, A. Ruzsinszky, P. Hao, Y.-S. Kim, G. Kresse, and J. P. Perdew, Physical Review B **84**, 035117 (2011).
[9] Z.-h. Yang, H. Peng, J. Sun, and J. P. Perdew, Physical Review B **93**, 205205 (2016).
[10] J. P. Perdew, W. Yang, K. Burke, Z. Yang, E. K. Gross, M. Scheffler, G. E. Scuseria, T. M. Henderson, I. Y. Zhang, A. Ruzsinszky, *et al.*, Proceedings of the National Academy of Sciences **114**, 2801 (2017).
[11] Y. Zhao and D. G. Truhlar, The Journal of chemical physics **125**, 194101 (2006).
[12] J. Tao, J. P. Perdew, V. N. Staroverov, and G. E. Scuseria, Physical Review Letters **91**, 146401 (2003).
[13] J. P. Perdew, A. Ruzsinszky, G. I. Csonka, L. A. Constantin, and J. Sun, Physical Review Letters **103**, 026403 (2009).
[14] J. Sun, B. Xiao, Y. Fang, R. Haunschild, P. Hao, A. Ruzsinszky, G. I. Csonka, G. E. Scuseria, and J. P. Perdew, Physical review letters **111**, 106401 (2013).
[15] S. Uchida, T. Ido, H. Takagi, T. Arima, Y. Tokura, and S. Tajima, Physical Review B **43**, 7942 (1991).
[16] C. Ye, P. Cai, R. Yu, X. Zhou, W. Ruan, Q. Liu, C. Jin, and Y. Wang, Nature communications **4**, 1365 (2013).
[17] S. Ono, S. Komiya, and Y. Ando, Physical Review B **75**, 024515 (2007).
[18] T. Das, R. Markiewicz, and A. Bansil, Physical Review B **81**, 174504 (2010).
[19] J. M. Tranquada, in *Handbook of High-Temperature Superconductivity* (Springer, 2007) pp. 257–298.
[20] D. Vaknin, S. K. Sinha, D. E. Moncton, D. C. Johnston, J. M. Newsam, C. R. Safinya, and H. E. King, Physical Review Letters **58**, 2802 (1987).
[21] K. Hirakawa and H. Ikeda, Physical Review Letters **33**, 374 (1974).
[22] S. Mitsuda, G. Shirane, S. Sinha, D. Johnston, M. Alvarez, D. Vaknin, and D. Moncton, Physical Review B **36**, 822 (1987).
[23] G. Shirane, Y. Endoh, R. Birgeneau, M. Kastner, Y. Hidaka, M. Oda, M. Suzuki, and T. Murakami, Physical review letters **59**, 1613 (1987).
[24] K. Yamada, E. Kudo, Y. Endoh, Y. Hidaka, M. Oda, M. Suzuki, and T. Murakami, Solid state communications **64**, 753 (1987).
[25] J. Akimitsu and Y. Ito, Journal of the Physical Society of Japan **40**, 1621 (1976).
[26] T. Freltoft, G. Shirane, S. Mitsuda, J. P. Remeika, and A. S. Cooper, Physical Review B **37**, 137 (1988).
[27] K. Yamada, K. Kakurai, Y. Endoh, T. Thurston, M. Kastner, R. Birgeneau, G. Shirane, Y. Hidaka, and T. Murakami, Physical Review B **40**, 4557 (1989).
[28] J. D. Jorgensen, B. Dabrowski, S. Pei, D. G. Hinks, L. Soderholm, B. Morosin, J. E. Schirber, E. L. Venturini, and D. S. Ginley, Physical Review B **38**, 11337 (1988).
[29] D. M. Ginsberg, *Physical properties of high temperature superconductors II* (World Scientific, 1998).
[30] E. S. Bozin, R. Zhong, K. R. Knox, G. Gu, J. P. Hill, J. M. Tranquada, and S. J. Billinge, Physical Review B **91**, 054521 (2015).
[31] J. Fink, N. Nucker, H. Romberg, and J. Fuggle, IBM Journal of Research and Development **33**, 372 (1989).
[32] C. Rao and B. Raveau, *Transition Metal Oxides: Structure, Properties, and Synthesis of Ceramic Oxides* (Wiley, 1998).
[33] A. Oleś, Physical Review B **28**, 327 (1983).
[34] Note, in the AFM unit cell the projected $d_{yz}$ and $d_{xz}$ orbitals do not align along the Cu-O bond and should be considered a linear combination of their aligned counterparts. However, this basis-set effect is averaged out and we find the same average spin-splitting.
